# Supplementary material for: Repairing and Mechanising the JavaScript Relaxed Memory Model
Source: arXiv:2005.10554 source file (2020-05-22)
Supplement: Supplementary file 1 [file appendix.tex]

%!TEX root = main.tex
\pagebreak
\appendix
\onecolumn
\section{Appendix}

\subsection{JavaScript Well-formedness}
\label{sec:app-wf}

%!TEX root = ../main.tex

\begin{figure*}[h]

\begin{tabular}{rcl@{\qquad}rcl}
$\func{range}_r(\obj{E}$ : \evttype) & $\triangleq$ & [ \obj{E}.\fld{index} \ldots $\obj{E}.\fld{index} + |\obj{E}.\fld{reads}|$ ) & $\func{read}(\obj{E}$ : \evttype) & $\triangleq$ & $(\obj{E}.\fld{reads} \neq [])$ \\
$\func{range}_w(\obj{E}$ : \evttype) & $\triangleq$ & [ \obj{E}.\fld{index} \ldots $\obj{E}.\fld{index} + |\obj{E}.\fld{writes}|$ ) & $\func{write}(\obj{E}$ : \evttype) & $\triangleq$ & $(\obj{E}.\fld{writes} \neq [])$ \\
$\func{range}(\obj{E}$ : \evttype) & $\triangleq$ & $\func{range}_r(\obj{E}) \cup \func{range}_w(\obj{E})$ & $\func{rmw}(\obj{E}$ : \evttype) & $\triangleq$ & $\func{read}(\obj{E}) \wedge \func{write}(\obj{E})$ \\
$\func{overlap}(\obj{E}_1, \obj{E}_2$ : \evttype)& $\triangleq$ & $\obj{E}_1.\fld{block} = \obj{E}_2.\fld{block}~\wedge$ &
$\func{read}(\obj{Es}$ : \settype{\evttype}) & $\triangleq$ & $\{  \obj{E} ~|~ \obj{E} \in \obj{Es} \wedge\func{read}(\obj{E}) \}$ \\
&&$\quad\func{range}(\obj{E}_1) \cap \func{range}(\obj{E}_2) \neq \emptyset$&
$\func{write}(\obj{Es}$ : \settype{\evttype}) & $\triangleq$ & $\{  \obj{E} ~|~ \obj{E} \in \obj{Es} \wedge\func{write}(\obj{E}) \}$
\vspace{0.5em}
\end{tabular}\\[0.2\baselineskip]

\begin{minipage}{0.565\textwidth}
\begin{tabular}{@{}l}
$\func{well-formed}(k : \nattype, \obj{E}_w : \evttype, \obj{E}_r : \evttype) \triangleq$\\
$\qquad k \in \func{range}_w(\obj{E}_w) \wedge k \in \func{range}_r(\obj{E}_r) \wedge \obj{E}_w.\fld{block} = \obj{E}_r.\fld{block}~\wedge$\\
$\qquad (\obj{E}_w.\fld{writes})!(k - \obj{E}_w.\fld{index}) = (\obj{E}_r.\fld{reads})!(k - \obj{E}_r.\fld{index}) \wedge \obj{E}_w \neq \obj{E}_r$
\end{tabular}
\end{minipage}%
\begin{minipage}{0.435\textwidth}
\raggedleft
\end{minipage}\\[0.7\baselineskip]

\begin{minipage}{0.565\textwidth}
\begin{tabular}{@{}l}
$\func{well-formed}(\obj{rbf}$ : $\settype{(\nattype \times \evttype \times \evttype)}, \obj{Es} : \settype{\evttype}) \triangleq$\\
$\qquad (~\forall \obj{E}_r \in \obj{Es}, k \in \func{range}_r(\obj{E}_r) \ldotp \exists! \obj{E}_w \ldotp \xxtriple{k}{\obj{E}_w}{\obj{E}_r} \in \obj{rbf}~)~\wedge$\\
$\qquad (~\forall \obj{E}_r \in \obj{Es}, k \notin \func{range}_r(\obj{E}_r) \ldotp \nexists \obj{E}_w \ldotp \xxtriple{k}{\obj{E}_w}{\obj{E}_r} \in \obj{rbf}~)~\wedge$\\
$\qquad \forall \xxtriple{k}{\obj{E}_w}{\obj{E}_r}  \in \obj{rbf} \ldotp \func{well-formed}(k,\obj{E}_w,\obj{E}_r)$
\end{tabular}
\end{minipage}%
\begin{minipage}{0.435\textwidth}
\begin{tabular}{@{}l}
$\func{well-formed}(\obj{CE} : \candidatetype) \triangleq$ \\
\qquad$\obj{CE}.\tot$ is a strict total order on $\obj{CE}.\fld{evs}~\wedge$\\
\qquad$\func{well-formed}(\obj{CE}.\rbf, \obj{CE}.\fld{evs})$\\
\\
\end{tabular}
\end{minipage}

\vspace{-0.5\baselineskip}
\caption{Candidate Execution Well-formedness}
\label{fig:candidate-execution-wf}
\vspace{-0.5\baselineskip}
\end{figure*}

\subsection{Comparison to Prose JavaScript Specification}
\label{sec:app-prose}

% \todocp{The following two subsections breaks the flow a bit. We could end the previous subsection by saying we'll look at this deficiency before briefly commenting on how the formal spec compares with the prose spec. But then 2.3 comes and it's not so clear where it's going.}
%
The model as presented by the paper is intended to be a faithful rendering in
logic of the model as it is described in the JavaScript specification.
However, we sometimes factor or name definitions differently for the
sake of a simpler presentation or to match standard terminology in the
literature.
Noticeable differences are highlighted here.

\begin{itemize}
\item The prose specification refers to written values as an event's ``payload''. Read events do not contain a payload field, but their read value is contained in a separate ``chosen value record''.
We simply make both of these fields part of the event as explicit read/write fields.

\item The prose specification uses the term
\rel{memory-order} to refer to what we call \rel{total-order}, but
this invites confusion with the C/C++11 memory model: there a ``memory
order'' is what JavaScript calls a ``consistency mode'', and
``$\rel{mo}$'' refers to ``modification order'', a per-location-total
order on writes~\cite{Batty:2011}.

\item In addition, the prose specification existentially quantifies \totr~as part of its validity conditions.
We make this a field of the candidate execution.

 \item
The prose specification does not make a distinction between well-formedness conditions (which are purely invariants of the thread-local semantics),
and validity conditions, which are semantic conditions imposed by the axiomatic memory model. We separate
well-formedness from validity in our rendering of the model because in
later sections we explicitly want to reason about executions which are
well-formed but nevertheless not valid.

\item In the prose specification our Happens-Before Consistency (2-3) conditions are collectively named the ``Coherent Reads'' condition.

\item In several cases, the prose specification defines predicates using a pseudocode algorithm.
For example, the prose specification's ``Coherent Reads'' condition is defined as an explicit iteration over the set of events, accumulating a boolean result, instead of as a more abstract universal quantification.

Our Happens-Before Consistency (1) condition is instead given as a component of Sequentially Consistent Atomics.

\item
The prose specification describes an additional condition that all
atomic writes must have a finite prefix in \tot.
This condition is vacuously true in real candidate executions, since \tot must be well-founded (every thread must have a first event in \seqb-order).
This condition is occasionally included in formal relaxed memory models as a well-formedness condition that is implied by the thread-local semantics~\cite{Batty:2011}.
However, we never need to use it, so we simply elide it here.

\end{itemize}

\subsection{Comparison to Alloy/Coq models}
As previously detailed, our proofs assume that all initialization happens ``before time''.
The Coq model undergoes two minor refactorings in order to better interface with the existing IMM models.
First, validity conditions have individual edges reversed so that they can be expressed as equivalent acyclicity constraints.
Second, RMW events are equivalently represented as two events which are always adjacent in \seqbr~and \totr.
Both of these transformations are analogous to the transformations made to other models (such as C/C++11) in previous works in order to simplify formal proofs~\cite{Lahav:2017:RSC:3062341.3062352, Moiseenko-al:CoRR19}

\section{ARMv8 model}
\label{arm_appendix}

%!TEX root = ../main.tex

\begin{tabular}{rcl@{~}l@{~}l}
$\type{mode}$ & $::=$ & \multicolumn{3}{l}{ $\tcons{ReadAcquire}$} \\
  & $|$ & \multicolumn{3}{l}{$\tcons{ReadWeakAcquire}$} \\
  & $|$ & \multicolumn{3}{l}{$\tcons{WriteRelease}$} \\
  & $|$ & \multicolumn{3}{l}{$\tcons{DMB.SY}$} \\
  & $|$ & \multicolumn{3}{l}{$\tcons{DMB.LD}$} \\
  & $|$ & \multicolumn{3}{l}{$\tcons{DMB.ST}$} \\
  & $|$ & \multicolumn{3}{l}{$\tcons{ISB}$} \\

$\type{addr}$ & $::=$ & \multicolumn{3}{l}{$\alpha \ldots $ an infinite set of abstract names} \\
%% \end{tabular}

%% \begin{tabular}{rcl@{~}l@{~}l}
$\type{event}$ & $::=$ &  \{ &  \fld{ord} & : \type{mode} \\
&&& \fld{index} & : \type{nat} \\
&&& \fld{reads} & : $\listtype{\bytetype}$ \\
&&& \fld{writes} & : $\listtype{\bytetype}$ \\

  $\candidatetype$ & $::=$ &  \{ & \fld{evs} & : $\settype{\evttype}$ \\
&&& \IW & : $\evttype$ \\
&&& \text{\po~\CMMT~\por} & : $\settype{(\nattype \times \evttype \times \evttype)}$ \\
&&& \text{\rbf~\CMMT~\rbfr} & : $\settype{(\nattype \times \evttype \times \evttype)}$ \\
  &&& \text{\cob~\CMMT~\cobr} & : $\settype{(\nattype \times \evttype \times \evttype)}$ \\
  &&& \text{\addrP~\CMMT~\addrPr} & : $\settype{(\evttype \times \evttype)}$ \\
  &&& \text{\dataP~\CMMT~\dataPr} & : $\settype{(\evttype \times \evttype)}$ \\
  &&& \text{\ctrlP~\CMMT~\ctrlPr} & : $\settype{(\evttype \times \evttype)}$ \\
  &&& \text{\rmw~\CMMT~\rmwr} & : $\settype{(\evttype \times \evttype)}$
  \} \\
\\
\end{tabular}

\raggedright
Following herd \cite{Alglave:2014}, we define relational composition ``$;$''
the identity relation ``[A]'' on a set $A$:
\begin{align*}
R; S \triangleq & \{ \xxpair{\obj{A}}{\obj{B}} \mid \exists \obj{C} \ldotp \xxpair{\obj{A}}{\obj{C}} \in R \land \xxpair{\obj{C}}{\obj{B}} \in S \} \\
[ E ] \triangleq & \{ \xxpair{\obj{E}}{\obj{E}} \mid \obj{E} \in A \}
\end{align*}

Then, $[A];R;[B]$ is the relation $R$ restricted to elements from $A$ on the left and elements from $B$ from the right:
$$
[A];R;[B] = \{ \xxpair{a}{b} \mid \xxpair{a}{b} \in R \land a \in A \land b \in B \}
$$

\paragraph{Derived auxiliary relations} \textit{(with respect to a candidate execution)}

\begin{align*}
  \sthd~\CMMT~\sthdr \triangleq &
  \{ \xxpair{\obj{A}}{\obj{B}} \mid 
  \xxpair{\obj{A}}{\obj{B}} \in \por \lor \xxpair{\obj{B}}{\obj{A}} \in \por \}
\\
  \rf~\CMMT~\rfr \triangleq & \{ \xxpair{\obj{A}}{\obj{B}} \mid \exists k \ldotp \xxtriple{k}{\obj{A}}{\obj{B}} \in \rbf \}
\\
  \co~\CMMT~\cor \triangleq &
  \{ \xxpair{\obj{A}}{\obj{B}} \mid \exists k \ldotp \xxtriple{k}{\obj{A}}{\obj{B}} \in \cob \}^+
\\
  \rfi~\CMMT~\rfir \triangleq & \rf \cap \sthd
\\
  \rfe~\CMMT~\rfer \triangleq &
  \rf \setminus \rfi
\\
  \coi~\CMMT~\coir \triangleq &
  \co \cap \sthd
\\
  \coe~\CMMT~\coer \triangleq &
  \co \setminus \coi
\\
  \frb~\CMMT~\frbr \triangleq &
  \{ \xxtriple{k}{\obj{A}}{\obj{B}} \mid \exists C \ldotp \xxtriple{k}{\obj{C}}{\obj{A}} \in \rbf \land \xxtriple{k}{\obj{C}}{\obj{B}} \in \cob \}^+
\\
  \fr~\CMMT~\frr \triangleq &
  \{ \xxpair{\obj{A}}{\obj{B}} \mid \exists k \ldotp \xxtriple{k}{\obj{A}}{\obj{B}} \in \frb \}^+
\\
  \fri~\CMMT~\frir \triangleq &
  \fr \cap \sthd
\\
  \fre~\CMMT~\frer \triangleq &
  \fr \setminus \fri 
\\
  \polocb~\CMMT~\polocbr \triangleq &
  \{ \xxtriple{k}{\obj{A}}{\obj{B}} \mid \xxpair{\obj{A}}{\obj{B}} \in \por \land k \in \func{range}(\obj{A}) \land k \in \func{range}(\obj{B}) \}
\\
\displaybreak
\\
\R \triangleq & \{ \obj{E} \mid \obj{E}.\fld{reads} \neq [] \} \\
\W \triangleq & \{ \obj{E} \mid \obj{E}.\fld{writes} \neq [] \} \\
\A \triangleq & \{ \obj{E} \mid \obj{E}.\fld{ord} = \tcons{ReadAcquire} \} \\
\Q \triangleq & \{ \obj{E} \mid \obj{E}.\fld{ord} = \tcons{ReadWeakAcquire} \} \\
\L \triangleq & \{ \obj{E} \mid \obj{E}.\fld{ord} = \tcons{WriteRelease} \} \\
\DMBSY \triangleq & \{ \obj{E} \mid \obj{E}.\fld{ord} = \tcons{DMB.SY} \} \\
\DMBLD \triangleq & \{ \obj{E} \mid \obj{E}.\fld{ord} = \tcons{DMB.LD} \} \\
\DMBST \triangleq & \{ \obj{E} \mid \obj{E}.\fld{ord} = \tcons{DMB.ST} \} \\
\ISB \triangleq & \{ \obj{E} \mid \obj{E}.\fld{ord} = \tcons{ISB} \} \\
\B \triangleq & \DMBSY \cup \DMBLD \cup \DMBST \cup \ISB \\
\\
\\
\addr~\CMMT~\addrr \triangleq & [R]; \addrPr \\
\data~\CMMT~\datar \triangleq & [R]; \dataPr \\
\ctrl~\CMMT~\ctrlr \triangleq & [R]; \ctrlPr \\
\\
\\
\ca~\CMMT~\car \triangleq &
  \cor \cup \frr
  \\
  \obs~\CMMT~\obsr \triangleq &
  \rfer \cup \frer \cup \coer
  \\
  \\
  \dob~\CMMT~\dobr \triangleq & \addrr \cup  \\
  &  \datar \cup \\
  &  (\ctrlr ; [\W]) \cup \\
  &  ((\ctrlr \cup \addrr; \por) ; [\ISB]; \por; [\R]) \cup \\
  &  (\addrr; \por ; [\W]) \cup \\
  &  ((\ctrlr \cup \datar); \coir)) \cup \\
  &  ((\addrr \cup \datar); \rfir))
\\
  \aob~\CMMT~\aobr \triangleq & \rmwr \cup (\rmwr;[R];\rfir;[\A \cup \Q])
\\
  \bob~\CMMT~\bobr \triangleq & \por;[\DMBSY];\por \cup \\
  & ([\LLL]; \por; [\A]) \cup \\
  & ([\R]; \por; [\DMBLD]; \por) \cup \\
  & ([\A \cup \Q]; \por) \cup \\
  & ([\W]; \por; [\DMBST]; \por; [\W]) \cup \\
  & (\por; [\LLL]) \cup \\
  & (\por; [\LLL]; \coir) \cup \\
\\
  \iob~\CMMT~\iobr \triangleq & \{ (\IW,E) \mid E \in \EV \setminus \IW \} \\
\\
  \ob~\CMMT~\obr \triangleq & \obsr \cup \dobr \cup \aobr \cup \bobr \\
\end{align*}

\paragraph{Well-formedness conditions}\hfill

Let $R_k$, for some relation $R : \settype{(\nattype \times \evttype \times \evttype)}$, denote the relation
$\{ \xxpair{A}{B} \mid \xxtriple{k}{A}{B} \in R \} : \settype{(\evttype \times \evttype)}$.

\begin{itemize}
\item The initial write is not a release write:
$$ \IW \subseteq W \setminus L $$

\item In our fragment, reads and writes are disjoint, and reads, writes, and barriers are disjoint:
$$\R \cap \W \cap \DMBSY \cap \DMBLD \cap DMBST \cap ISB = \emptyset$$

\item Barriers don't read or write memory:
$$\{ \func{range}(\obj{E}) \mid E \in \B \} = \emptyset$$

\item For all locations $k$, $\cobr_k$ is a strict total order on $\{ W \mid k \in W.\fld{writes} \}$ $\dots$

\item $\dots$ and only includes writes that write to $k$:
$$ \forall k, W, W'. \xxpair{W}{W'} \in \cobr_k \implies k \in W.\fld{writes} \cap W'.\fld{writes}$$

\item $\co$ is a strict partial order.

\item $\rmw$, $\addr$, $\data$, and $\ctrl$ are subsets of $\po$:
$$\rmwr \cup \addrr \cup \datar \cup \ctrlr \subseteq \por$$

\end{itemize}

\paragraph{Candidate execution validity}\hfill

\vspace{2em}

\textbf{Single-copy atomicity}\\
$(\rfr; \frr) \ \text{irreflexive}$

\vspace{1em}

\textbf{Coherence/internal}\\
$\forall k. (\polocbr_k \cup \frbr_k \cup \cobr_k \cup \rbfr_k) \ \text{acyclic}$

\vspace{1em}

\textbf{External}\\
$\obr \ \text{acyclic}$

\vspace{1em}

\textbf{Exclusives/Atomic}\\
$\rmwr \cap (\frer; \coer) = \emptyset$
