# Supplementary material for: Repairing and Mechanising the JavaScript Relaxed Memory Model
Source: arXiv:2005.10554 source file (2020-05-22)
Supplement: Supplementary file 2 [file arm_appendix.tex]

%!TEX root = ../main.tex

\begin{tabular}{rcl@{~}l@{~}l}
$\type{mode}$ & $::=$ & \multicolumn{3}{l}{ $\tcons{ReadAcquire}$} \\
  & $|$ & \multicolumn{3}{l}{$\tcons{ReadWeakAcquire}$} \\
  & $|$ & \multicolumn{3}{l}{$\tcons{WriteRelease}$} \\
  & $|$ & \multicolumn{3}{l}{$\tcons{DMB.SY}$} \\
  & $|$ & \multicolumn{3}{l}{$\tcons{DMB.LD}$} \\
  & $|$ & \multicolumn{3}{l}{$\tcons{DMB.ST}$} \\
  & $|$ & \multicolumn{3}{l}{$\tcons{ISB}$} \\

$\type{addr}$ & $::=$ & \multicolumn{3}{l}{$\alpha \ldots $ an infinite set of abstract names} \\
%% \end{tabular}

%% \begin{tabular}{rcl@{~}l@{~}l}
$\type{event}$ & $::=$ &  \{ &  \fld{ord} & : \type{mode} \\
&&& \fld{index} & : \type{nat} \\
&&& \fld{reads} & : $\listtype{\bytetype}$ \\
&&& \fld{writes} & : $\listtype{\bytetype}$ \\

  $\candidatetype$ & $::=$ &  \{ & \fld{evs} & : $\settype{\evttype}$ \\
&&& \IW & : $\evttype$ \\
&&& \text{\po~\CMMT~\por} & : $\settype{(\nattype \times \evttype \times \evttype)}$ \\
&&& \text{\rbf~\CMMT~\rbfr} & : $\settype{(\nattype \times \evttype \times \evttype)}$ \\
  &&& \text{\cob~\CMMT~\cobr} & : $\settype{(\nattype \times \evttype \times \evttype)}$ \\
  &&& \text{\addrP~\CMMT~\addrPr} & : $\settype{(\evttype \times \evttype)}$ \\
  &&& \text{\dataP~\CMMT~\dataPr} & : $\settype{(\evttype \times \evttype)}$ \\
  &&& \text{\ctrlP~\CMMT~\ctrlPr} & : $\settype{(\evttype \times \evttype)}$ \\
  &&& \text{\rmw~\CMMT~\rmwr} & : $\settype{(\evttype \times \evttype)}$
  \} \\
\\
\end{tabular}

\raggedright
Following herd \cite{Alglave:2014}, we define relational composition ``$;$''
the identity relation ``[A]'' on a set $A$:
\begin{align*}
R; S \triangleq & \{ \xxpair{\obj{A}}{\obj{B}} \mid \exists \obj{C} \ldotp \xxpair{\obj{A}}{\obj{C}} \in R \land \xxpair{\obj{C}}{\obj{B}} \in S \} \\
[ E ] \triangleq & \{ \xxpair{\obj{E}}{\obj{E}} \mid \obj{E} \in A \}
\end{align*}

Then, $[A];R;[B]$ is the relation $R$ restricted to elements from $A$ on the left and elements from $B$ from the right:
$$
[A];R;[B] = \{ \xxpair{a}{b} \mid \xxpair{a}{b} \in R \land a \in A \land b \in B \}
$$

\paragraph{Derived auxiliary relations} \textit{(with respect to a candidate execution)}

\begin{align*}
  \sthd~\CMMT~\sthdr \triangleq &
  \{ \xxpair{\obj{A}}{\obj{B}} \mid 
  \xxpair{\obj{A}}{\obj{B}} \in \por \lor \xxpair{\obj{B}}{\obj{A}} \in \por \}
\\
  \rf~\CMMT~\rfr \triangleq & \{ \xxpair{\obj{A}}{\obj{B}} \mid \exists k \ldotp \xxtriple{k}{\obj{A}}{\obj{B}} \in \rbf \}
\\
  \co~\CMMT~\cor \triangleq &
  \{ \xxpair{\obj{A}}{\obj{B}} \mid \exists k \ldotp \xxtriple{k}{\obj{A}}{\obj{B}} \in \cob \}^+
\\
  \rfi~\CMMT~\rfir \triangleq & \rf \cap \sthd
\\
  \rfe~\CMMT~\rfer \triangleq &
  \rf \setminus \rfi
\\
  \coi~\CMMT~\coir \triangleq &
  \co \cap \sthd
\\
  \coe~\CMMT~\coer \triangleq &
  \co \setminus \coi
\\
  \frb~\CMMT~\frbr \triangleq &
  \{ \xxtriple{k}{\obj{A}}{\obj{B}} \mid \exists C \ldotp \xxtriple{k}{\obj{C}}{\obj{A}} \in \rbf \land \xxtriple{k}{\obj{C}}{\obj{B}} \in \cob \}^+
\\
  \fr~\CMMT~\frr \triangleq &
  \{ \xxpair{\obj{A}}{\obj{B}} \mid \exists k \ldotp \xxtriple{k}{\obj{A}}{\obj{B}} \in \frb \}^+
\\
  \fri~\CMMT~\frir \triangleq &
  \fr \cap \sthd
\\
  \fre~\CMMT~\frer \triangleq &
  \fr \setminus \fri 
\\
  \polocb~\CMMT~\polocbr \triangleq &
  \{ \xxtriple{k}{\obj{A}}{\obj{B}} \mid \xxpair{\obj{A}}{\obj{B}} \in \por \land k \in \func{range}(\obj{A}) \land k \in \func{range}(\obj{B}) \}
\\
\displaybreak
\\
\R \triangleq & \{ \obj{E} \mid \obj{E}.\fld{reads} \neq [] \} \\
\W \triangleq & \{ \obj{E} \mid \obj{E}.\fld{writes} \neq [] \} \\
\A \triangleq & \{ \obj{E} \mid \obj{E}.\fld{ord} = \tcons{ReadAcquire} \} \\
\Q \triangleq & \{ \obj{E} \mid \obj{E}.\fld{ord} = \tcons{ReadWeakAcquire} \} \\
\L \triangleq & \{ \obj{E} \mid \obj{E}.\fld{ord} = \tcons{WriteRelease} \} \\
\DMBSY \triangleq & \{ \obj{E} \mid \obj{E}.\fld{ord} = \tcons{DMB.SY} \} \\
\DMBLD \triangleq & \{ \obj{E} \mid \obj{E}.\fld{ord} = \tcons{DMB.LD} \} \\
\DMBST \triangleq & \{ \obj{E} \mid \obj{E}.\fld{ord} = \tcons{DMB.ST} \} \\
\ISB \triangleq & \{ \obj{E} \mid \obj{E}.\fld{ord} = \tcons{ISB} \} \\
\B \triangleq & \DMBSY \cup \DMBLD \cup \DMBST \cup \ISB \\
\\
\\
\addr~\CMMT~\addrr \triangleq & [R]; \addrPr \\
\data~\CMMT~\datar \triangleq & [R]; \dataPr \\
\ctrl~\CMMT~\ctrlr \triangleq & [R]; \ctrlPr \\
\\
\\
\ca~\CMMT~\car \triangleq &
  \cor \cup \frr
  \\
  \obs~\CMMT~\obsr \triangleq &
  \rfer \cup \frer \cup \coer
  \\
  \\
  \dob~\CMMT~\dobr \triangleq & \addrr \cup  \\
  &  \datar \cup \\
  &  (\ctrlr ; [\W]) \cup \\
  &  ((\ctrlr \cup \addrr; \por) ; [\ISB]; \por; [\R]) \cup \\
  &  (\addrr; \por ; [\W]) \cup \\
  &  ((\ctrlr \cup \datar); \coir)) \cup \\
  &  ((\addrr \cup \datar); \rfir))
\\
  \aob~\CMMT~\aobr \triangleq & \rmwr \cup (\rmwr;[R];\rfir;[\A \cup \Q])
\\
  \bob~\CMMT~\bobr \triangleq & \por;[\DMBSY];\por \cup \\
  & ([\LLL]; \por; [\A]) \cup \\
  & ([\R]; \por; [\DMBLD]; \por) \cup \\
  & ([\A \cup \Q]; \por) \cup \\
  & ([\W]; \por; [\DMBST]; \por; [\W]) \cup \\
  & (\por; [\LLL]) \cup \\
  & (\por; [\LLL]; \coir) \cup \\
\\
  \iob~\CMMT~\iobr \triangleq & \{ (\IW,E) \mid E \in \EV \setminus \IW \} \\
\\
  \ob~\CMMT~\obr \triangleq & \obsr \cup \dobr \cup \aobr \cup \bobr \\
\end{align*}

\paragraph{Well-formedness conditions}\hfill

Let $R_k$, for some relation $R : \settype{(\nattype \times \evttype \times \evttype)}$, denote the relation
$\{ \xxpair{A}{B} \mid \xxtriple{k}{A}{B} \in R \} : \settype{(\evttype \times \evttype)}$.

\begin{itemize}
\item The initial write is not a release write:
$$ \IW \subseteq W \setminus L $$

\item In our fragment, reads and writes are disjoint, and reads, writes, and barriers are disjoint:
$$\R \cap \W \cap \DMBSY \cap \DMBLD \cap DMBST \cap ISB = \emptyset$$

\item Barriers don't read or write memory:
$$\{ \func{range}(\obj{E}) \mid E \in \B \} = \emptyset$$

\item For all locations $k$, $\cobr_k$ is a strict total order on $\{ W \mid k \in W.\fld{writes} \}$ $\dots$

\item $\dots$ and only includes writes that write to $k$:
$$ \forall k, W, W'. \xxpair{W}{W'} \in \cobr_k \implies k \in W.\fld{writes} \cap W'.\fld{writes}$$

\item $\co$ is a strict partial order.

\item $\rmw$, $\addr$, $\data$, and $\ctrl$ are subsets of $\po$:
$$\rmwr \cup \addrr \cup \datar \cup \ctrlr \subseteq \por$$

\end{itemize}

\paragraph{Candidate execution validity}\hfill

\vspace{2em}

\textbf{Single-copy atomicity}\\
$(\rfr; \frr) \ \text{irreflexive}$

\vspace{1em}

\textbf{Coherence/internal}\\
$\forall k. (\polocbr_k \cup \frbr_k \cup \cobr_k \cup \rbfr_k) \ \text{acyclic}$

\vspace{1em}

\textbf{External}\\
$\obr \ \text{acyclic}$

\vspace{1em}

\textbf{Exclusives/Atomic}\\
$\rmwr \cap (\frer; \coer) = \emptyset$
